# Supplementary material for: Raccoon: Multi-stage Diffusion Training with Coarse-to-Fine Curating Videos
Source: arXiv:2502.21314 source file (2025-03-07)
Supplement: Supplementary file 1 [file supp.tex]

\section{Ethical and Social Impacts}

Our work in text-based HIG using the HcP layer, which relies on reference images sourced from publicly available datasets and base models publicly released on the HuggingFace diffusers library \cite{von2022diffusers}, presents various ethical and social considerations.
The primary concern is the potential impact on privacy and data protection. The generation of human images based on text inputs could unintentionally produce likenesses of real individuals, highlighting the need for guidelines to protect individual privacy and meanwhile prevent misuse of personal likenesses. Additionally, the inherited biases in the training datasets and base models can lead to stereotypical images. It's important to continuously monitor and adjust these biases to ensure a fair and inclusive representation of generated human figures.

Furthermore, while our method can enhance representation in digital media by generating diverse and accurate human figures, there is a risk of misuse in creating misleading or harmful content. Establishing ethical guidelines and usage policies is crucial to prevent the creation of deepfakes. Collaborative efforts with various stakeholders are necessary to develop responsible use cases and address potential misuse.
In summary, our approach in tHIG, while offering the potential for creative and inclusive image generation, must be balanced with a commitment to ethical practices, privacy protection, and the promotion of diversity and inclusivity in text-based human figure synthesis.

\section{Cross-Attention Layer Details}

The cross-attention layer within the U-Net architecture of latent diffusion models plays a pivotal role in synthesizing detailed and contextually relevant images. This layer operates by computing a set of queries ($\mathbf{Q}$), keys ($\mathbf{K}$), and values ($\mathbf{V}$) based on the input latent representation 
$\mathbf{z}_{in}$ and the given text-conditioned embeddings $\mathcal{C}$. 

First, the input latent representation $\mathbf{z}_{in} $is transformed into a query matrix $\mathbf{Q}$ using a weight matrix $\mathbf{W}_q$. This process converts the input into the query space:
\begin{equation}
    \mathbf{Q} = \mathbf{W}_q ~ \mathbf{z}_{in} \in \mathbb{R}^{d}~,
\end{equation}

Simultaneously, text-conditioned embeddings $\mathcal{C}$ from CLIP \cite{radford2021learning} text encoder, which embeds textual information, is used to generate the key $\mathbf{K}$ and value $\mathbf{V}$ matrices through their respective weight matrices $\mathbf{W}_k$and $\mathbf{W}_v$:
\begin{equation}
    \begin{aligned}
        \mathbf{K} &= \mathbf{W}_k ~ \mathcal{C} \in \mathbb{R}^{d \times N}~,\\
        \mathbf{V} &= \mathbf{W}_v ~ \mathcal{C} \in \mathbb{R}^{d \times N}~,\\
    \end{aligned}
\end{equation}

The attention mechanism then computes the attention map $\mathcal{M}$ by applying a softmax function to the dot product of $\mathbf{Q}$ and $\mathbf{K}^T$, scaled by the square root of the dimensionality $d$. This step effectively captures the relevance of each element in the context of the input latent representation:
\begin{equation}
    \mathcal{M} = \text{softmax} \left( \frac{\mathbf{Q} \mathbf{K}^T}{\sqrt{d}} \right)~,
    \label{equ:softmax}
\end{equation}

Finally, the output latent representation $\mathbf{z}_{out}$ is obtained by multiplying the value matrix $\mathbf{V}$ with a combined attention map $\hat{\mathcal{M}}$ in Eq.~\ref{equ:2}, which is an enhanced version of $\mathcal{M}$ incorporating the novel Human-centric Prior (HcP) layer introduced in our approach:
\begin{equation}
    \mathbf{z}_{out} = \mathbf{V} \times \hat{\mathcal{M}} \in \mathbb{R}^{d}~,
\end{equation}

This augmented cross-attention mechanism, through $\hat{\mathcal{M}}$, effectively integrates human-centric prior information into the diffusion process, leading to more accurate and detailed human image synthesis in the generated images.

\section{Detailed Experiment Settings}
\label{app: setting}
Following the work of Ju \etal \cite{ju2023humansd}, we train the HcP layer on the ensemble of LAION-Human, and the training set of Human-Art, and test on the validation set of Human-Art.
Note that we only apply the text-based prompt in the validation set for inference evaluation.

\mypara{Human-Art} \cite{ju2023humansd} contains 50k high-quality images with over 123k person instances from 5 natural and 15 artificial scenarios, which are annotated with bounding boxes, key points, self-contact points, and text information for humans represented in both 2D and 3D. It is, therefore, comprehensive and versatile for various downstream tasks.

In our study, we specifically focus on the \textit{real human} category of the Human-Art dataset, as it directly aligns with our goal of addressing human image generation challenges. This category encompasses five sub-categories: \textit{acrobatics}, \textit{dance}, \textit{drama}, \textit{cosplay}, and \textit{movie}. These sub-categories offer a diverse range of human actions and poses, providing an ideal context for training the HcP layer to handle complex human structures. Examples are shown in Figure \ref{fig:example}.

\begin{figure}[h]
\centering
    \includegraphics[width=\linewidth]{figs/humanart.pdf}
    \caption{\textbf{Example images from the \textit{realhuman} category in the Human-Art dataset.} Each sub-category (\textit{acrobatics}, \textit{dance}, \textit{drama}, \textit{cosplay}, and \textit{movie}) is represented by four distinct images.}
    \label{fig:example}
\end{figure}

\mypara{Laion-Human} \cite{ju2023humansd}.
Ju \etal also constructed a dataset LAION-Human containing large-scale internet images. Specifically, they collected about 1M image-text pairs from LAION-5B \cite{schuhmann2022laion} filtered by the rules of high image quality and high human estimation confidence scores. Superior to ControlNet,
a versatile pose estimator is trained on the Human-Art dataset, which allows for selecting more diverse images such as oil paintings and cartoons. Importantly, LAION-Human contains more diverse human actions and more photorealistic images than data used in ControlNet.

\mypara{Implementation Details}.
Detailed implementation settings of training \& inference stages are listed in Table \ref{tab:impd}. All experiments are performed on 8$\times$ Nvidia Tesla A100 GPUs.
\begin{table}[t]
    \centering
        \caption{List of implementation settings for both training and inference stages.}
    \begin{tabular}{l c  }
    \toprule
      Implementation   & Setting  \\
      \midrule
      Training Noise Schedular &  DDPM \cite{ho2020denoising} \\ 
        Epoch &  10 \\
        Batch size per GPU & 8 \\
        Optimizer &  Adam \\
        Learning rate & 0.0001  \\
        weight decay & 0.01  \\
        Attention map ratio $\gamma$ & 0.1  \\
        loss ratio $\alpha$ & 0.1  \\
        Training timestamp & 1000 \\
        Training image size & 512 $\times$ 512  \\
        Training pose image size & 256 $\times$ 256  \\
        \midrule
         Sampling Noise Schedular &  DDIM \cite{song2020denoising} \\
         Inference step &  50 \\
        guidance scale & 7.5 \\
        Inference image size & 512 $\times$ 512  \\
        \bottomrule
    \end{tabular}

    \label{tab:impd}
\end{table}

\section{Additional Ablations and Analyses}

\subsection{Attention Combination Weight $\gamma$}
In this analysis, we focused on the ratio of attention map combination in Eq.~\ref{equ:2} of the main text, as illustrated in Figure \ref{fig:gammavis}. This examination helps us understand the effects of different ratios on the generated images.
At lower ratios of 0.01 and 0.05, the images closely resemble those produced by the standard SD model, indicating that the Human-centric Prior (HcP) layer's adjustments are minimal and maintain the foundational characteristics of the SD outputs.
The most effective correction occurs at a ratio of 0.1, where the HcP layer's influence is well balanced, significantly enhancing the accuracy of human figure generation while maintaining the original style and content of the SD model.
However, a ratio of 0.2 leads to noticeable changes in both the content and style, diverging markedly from the SD model's outputs. Although this ratio corrects the human figures, it also significantly alters the overall image, affecting both the composition and thematic elements.
In conclusion, these observations highlight the importance of an appropriate ratio to achieve a balance between correcting structural inaccuracies and preserving the original style and content of the images. The 0.1 ratio emerges as the most effective, offering an optimal blend of correction and preservation.

\begin{figure}[t]
\centering
    \includegraphics[width=0.9\linewidth]{figs/ablation_gamma.pdf}
    \caption{\textbf{Illustration of varying ratios (0.01, 0.05, 0.1, and 0.2) in the attention map combination on image generation.} Images generated for the given prompt at varying attention map combination ratios (0.01, 0.05, 0.1, 0.2).}
    \label{fig:gammavis}
\end{figure}

\subsection{Learning Process with Pose Image}
Figure \ref{fig:pose} provides a visualization of the alignment between layer-specific ResNet features and corresponding scales of the human-centric attention map from the HcP layer. This visualization clearly demonstrates a notable similarity between the layer-specific ResNet features and the cross-attention maps at equivalent scales.
This alignment plays a crucial role in our methodology. By ensuring that the ResNet features, which contain human-centric information, are closely aligned with the corresponding scales of the cross-attention layers, we enhance the model's ability to accurately incorporate human-centric details into the image generation process. This approach not only improves the structural integrity of the generated human figures but also ensures a more contextually accurate representation.

\begin{figure}[h]
\centering
    \includegraphics[width=\linewidth]{figs/attn_map_hloss.pdf}
    \caption{\textbf{Illustration of alignment between layer-specific ResNet features with corresponding scales and combined attention maps in each cross-attention layer.} The ResNet features are extracted from four different scale layers of a ImageNet pre-trained ResNet50 model.}
    \label{fig:pose}
\end{figure}

\section{Additional Results}
Due to space limitations, we only provide parts of the results in the main paper. In this section, we will report additional additional results, details, and analyses.

\begin{figure}[t]
\centering
    \includegraphics[width=\linewidth]{figs/control_app.pdf}
    \caption{\textbf{Additional comparisons and compatibility with the controllable HIG application.} We selected ControlNet \cite{zhang2023adding} as the basic model for controllable HIG and utilized OpenPose image as the conditional input.}
    \label{fig:control_app}
\end{figure}

\subsection{Human Evaluation Details}
\label{app: human}
We provide the human evaluation setting details here. In the main text, we request participants to evaluate \emph{anatomy quality} (AQ) and \emph{text-image alignment} (TIA) for the prompt-generated image pairs. The former reflects viewers' experience in terms of the anatomical quality of the images. In contrast, the latter reflects viewers' subjective perceptions of text-image consistency between the generated images and corresponding text prompts.
Before rating, we explain the whole procedure of our model and present some example pairs. When displaying these pairs, we explain the definition of AQ and TIA to each participant for a more precise understanding. Pairs that they require to rate are not included in these examples.
Images are displayed in full-screen mode on calibrated 27-inch LED monitors (Dell P2717H). Viewing conditions are in accordance with the guidelines of international standard procedures for multimedia subjective testing~\cite{ITU}. The subjects are all university undergraduate or graduate students with at least two years of experience in image processing, and they claimed to browse images frequently. The percentage of female subjects is about 40\%. All the subjects are aged from 20 to 27 years old.
Before giving the final rating, we allow participants to watch each pair multiple times.

\subsection{Controllable HIG Comparison}
\label{app: controlnet}
We provide additional comparisons with ControlNet \cite{zhang2023adding} as shown in Figure \ref{fig:control_app}.
Note that in most cases, under the control of OpenPose images, ControlNet generates human images with the correct pose. The HcP layer does not interfere with generating human images with correct structures but acts to correct them in cases of errors. This makes the HcP layer an effective tool in preventing the generation of structurally incorrect human images.

\subsection{Human-centric Prior Information Comparison}
\label{app: depth}
We provide additional results with different sources of human-centric prior information in Figure \ref{fig:depth_app}.

\begin{figure}[t]
\centering
    \includegraphics[width=\linewidth]{figs/depth_app.pdf}
    \caption{\textbf{Additional comparisons by using different sources of human-centric prior information}. The HcP layer is trained consistently for both Pose and Depth priors to ensure a fair and balanced comparison.}
    \label{fig:depth_app}
\end{figure}

\subsection{Qualitative Results}
\label{app: qualitative}
We provide additional qualitative results with baseline methods on three example prompts in Figure \ref{fig:lora_app}, and
we also provide additional large diffusion model (SDXL) results on four example prompts in Figure \ref{fig:sdxl_app}.

\subsection{Failure Cases Analysis}

\begin{figure}[h]
\centering
    \includegraphics[width=\linewidth]{figs/basecase.pdf}
    \caption{\textbf{Failure cases in complex action scenarios.} Two examples are generated using a pre-trained SDXL-base and an SDXL-base with the integrated HcP layer, in response to a more complex scene text prompt.}
    \label{fig:control_app_fail}
\end{figure}

We examine two instances where the generation of images based on the prompt ``\textit{three people doing a break dance pose}" fell short of expectations in Figure~\ref{fig:control_app_fail}. The main reasons for these limitations are as follows. First, the generation of detailed facial features and limbs is less accurate. This inaccuracy may be due to the limitations of the SDXL-base model itself, particularly when depicting multiple individuals in a complex scene. Second, the intricacy of the `\textit{break dance}' action, combined with the presence of multiple individuals, makes it more challenging to maintain accurate human structure in the generated images.
Despite these challenges, it is noteworthy that the images generated with our HcP layer show improvements in human figure representation compared to those produced by the SDXL-base model. This highlights the HcP layer's effectiveness in enhancing image quality, even in complex scenarios involving detailed movements and multiple subjects.

\section{Futuer work}

Advancing from our present achievements, two crucial areas are highlighted for future development in text-based human image generation:

\mypara{Diverse Data Learning:} To improve the model's capability in handling complex scenarios, we plan to enrich our dataset with more varied and intricate human actions. This will enable continued learning and refinement, enabling better representation of dynamic human interactions.

\mypara{Broader Priors Integration:} We target to incorporate additional human-centric priors simultaneously, such as depth and edge, which will enhance the detail and realism of generated human figures, overcoming the limitations of relying solely on pose information.

\newpage
\begin{figure*}[t]
\centering
    \includegraphics[width=\linewidth]{figs/lora_app.pdf}
    \caption{\textbf{Additional qualitative comparison with baseline methods on three example prompts}. We leverage the pre-trained SD v1-5 model for both ``with LoRA" and ``with HcP" models while keeping it frozen.}
    \label{fig:lora_app}
\end{figure*}

\newpage
\begin{figure*}[t]
\centering
    \includegraphics[width=\linewidth]{figs/sdxl_app.pdf}
    \caption{\textbf{Additional results on larger diffusion model (SDXL-base) using HcP layer}. We leverage the pre-trained SDXL-base model for the ``with HcP" model while keeping it frozen.
    }
    \label{fig:sdxl_app}
\end{figure*}
